# Supplementary material for: Topological Planning with Transformers for Vision-and-Language Navigation
Source: arXiv:2012.05292 source file (2020-12-09)
Supplement: Supplementary file 1 [file supplemental.tex]

% \begin{algorithm}
% \SetAlgoLined
% \SetKwInOut{Input}{input}
% \SetKwInOut{Hyperparam}{param}
% \Input{$\{o_1,o_2,...,o_n\}$ panoramas at planned nodes }
% \Hyperparam{$\sigma^2$ variance of bias function \newline $d$ localization threshold}
%  $\phi'_0 \leftarrow \vec 1, k \leftarrow 1, t \leftarrow 1$, \sc{observe} $o_0$\\
%  \While{$k \le n$}{
%     \sc{observe} $o_{curr}$\\
%     $\phi_t,\rho_t \leftarrow C_{high}(o_{k-1}, o_{curr}, o_k)$ \\
%     \eIf{$\rho_t \le d$}{
%         $k \leftarrow k + 1$
%     }{
%         $\phi'_t \leftarrow B (\phi_t, \phi'_{t-1}; \sigma^2)$ \\
%         \sc{execute} $C_{low}(\arg\max_i \phi'_{t_i})$ \\
%         $t \leftarrow t+ 1$
%     }
%  }
%  \caption{Combined Controller Logic}
%  \label{alg:control-alg}
% \end{algorithm}

% \paragraph{Overfitting.} One observation that we found during our experiments was overfitting. Transformer models are often trained with large volumes of data \cite{devlin2018bert,radford2018improving,radford2019language,brown2020language,dosovitskiy2020image}. For example, GPT-3 was trained on billions of data samples \cite{brown2020language}, and the vision transformer only achieves high performance when trained on large datasets (14M-300M images), whereas using mid-sized image datasets resulted in modest accuracies \cite{dosovitskiy2020image}. In contrast, the VLN-CE dataset contains fewer than 11k episodes in the training set. It would be interesting to see how performance may change with more data.

% Difficulty recovering when it begins trajectory in wrong direction
% \paragraph{Challenges.} Main challenges with planner are:
% \begin{itemize}
%     \item Overfitting.
%     \item Not stopping at the right time.
%     \item Begins trajectory in wrong direction and fails to recover.
% \end{itemize}


% \begin{figure}[t]
% \begin{center}
%   \includegraphics[width=\linewidth]{figs/plan_success_control_success.png}
% \end{center}
%   \caption{Example of success, where planner correctly produces a path terminating at a node $\le 3m$ from the labeled goal, and controller successfully executes the plan.}
% \label{fig:polar-slice-gaussian}
% \end{figure}

% \begin{figure}[t]
% \begin{center}
%   \includegraphics[width=0.8\linewidth]{figs/failure_oracle_success.png}
% \end{center}
%   \caption{Example of oracle success, where the trajectory fails to terminate close to the goal, but agent has been within proximity to it.}
% \label{fig:polar-slice-gaussian}
% \end{figure}


% \begin{figure}[t]
% \begin{center}
%   \includegraphics[width=0.8\linewidth]{figs/planning_failure.png}
% \end{center}
%   \caption{Example of planning failure but controller success.}
% \label{fig:polar-slice-gaussian}
% \end{figure}


% \begin{figure}[t]
% \begin{center}
%   \includegraphics[width=0.8\linewidth]{figs/highly_ambiguous.png}
% \end{center}
%   \caption{Example of ambiguous text instruction. The environment has many archways.}
% \label{fig:polar-slice-gaussian}
% \end{figure}

% Mapping methods:
% \begin{itemize}
%     \item NTS GT
%     \item Local control
% \end{itemize}
% \begin{figure}[t]
% \begin{center}
%   \includegraphics[width=0.8\linewidth]{figs/Screen Shot 2020-09-30 at 9.09.25 PM.png}
% \end{center}
%   \caption{Example of caption.  It is set in Roman so that mathematics
%   (always set in Roman: $B \sin A = A \sin B$) may be included without an
%   ugly clash.}
% \label{fig:long}
% \label{fig:onecol}
% \end{figure}
% \begin{figure}[t]
% \begin{center}
%   \includegraphics[width=0.8\linewidth]{figs/Screen Shot 2020-10-13 at 4.22.58 PM.png}
% \end{center}
%   \caption{Example of caption.  It is set in Roman so that mathematics
%   (always set in Roman: $B \sin A = A \sin B$) may be included without an
%   ugly clash.}
% \label{fig:polar-slice-gaussian}
% \end{figure}
